# Supplementary material for: Correlating neural and symbolic representations of language
Source: arXiv:1905.06401 source file (2019-06-05)
Supplement: Supplementary file 1 [file appendix.tex]

\onecolumn
\begin{appendices}

\section*{Supplementary material}
\label{sec:supplement}

\paragraph{Tree Kernel algorithm}
Following \citet{collins2002convolution}, we calculate the tree kernel
between two trees $T_1$ and $T_2$ as:

    \begin{equation}
      K(T_1, T_2) = \sum_{n_1\in T_1}\sum_{n_2\in T_2} C(n_1, n_2, \lambda),
    \end{equation}
    where $n_1$ and $n_2$ are the complete sets of tree fragments in
    $T_1$ and $T_2$, respectively, and the function $ C(n_1, n_2,
    \lambda)$ is calculated as:

    \begin{equation}
      C(n_1, n_2, \lambda) =
      \begin{cases}
        0, & \mbox{if } \mathrm{prod}(n_1)\ne\mathrm{prod}(n_2) \\
        \lambda, & \mbox{if } \mathrm{preterm}(n_1) \land \mathrm{preterm}(n_2) \\
        \lambda * \prod_{i=1}^{\mathrm{nc}(n_1)} (1 + C(\mathrm{ch}(n_1, i), \mathrm{ch}(n_2, i), \lambda)) & \mbox{otherwise}.
      \end{cases}
    \end{equation}
Here $\mathrm{nc}(n)$ is the number of children of a given
    (sub)tree, and $\mathrm{ch}(n, i)$ is its i$^{th}$
    child; $\mathrm{prod}(n)$ is the production of node $n$, and
    $\mathrm{preterm}(n)$ is true if $n$ is a preterminal node.

\end{appendices}
